# Supplementary material for: Velocity Obstacle for Polytopic Collision Avoidance for Distributed Multi-robot Systems
Source: arXiv:2304.07954 source file (2024-06-10)
Supplement: Supplementary file 1 [file supplement.tex]

$-R=\big\{-r \big|r \in R \big\}$ denote the robot A reflect in its reference point.

extend the VO concept to polytope field to achieve collision avoidance for two polytopic robots.

including the which could be simply calculated by some external algorithm (e.g.,A* or RRT*). 

RL: but these approaches require state-of-the-art hardware embedded into the robot, which might be a limiting factor in some cases.

is also a variant of VO, compared to VO which describes an area when choosing a velocity inside it will result in collision, ORCA describes an area when choosing a velocity inside it could assure collision avoidance. 
What's more, in order to incorporate the non-holonomic constraints, \cite{alonso2013optimal} proposed Non-Holonomic ORCA (NH-ORCA) which combines the kinematic model with ORCA.

Instead of only a single robot takes the whole responsibility for collision avoidance just as VO, RVO let one robot only takes just half responsibility for collision avoidance and and the other robot take the other half to achieve reciprocal collision avoidance.
However, RVO also has some defects, it require both robots choose to pass each other from the same side of the respective RVO to assure collision avoidance and no oscillations known as "reciprocal dance"\cite{johnson2020colliding}.
This condition may not be guaranteed in the dense packed environment and will result in unnecessary oscillations known as "reciprocal dance".
was proposed to deal with the defect of RVO, it replaces the side which we don't want the robot to pass of RVO by the side of VO to make sure both robots choose to pass each other from the same side as much as possible.

The artificial potential field method, proposed in \cite{khatib1985real}, has been extended to account for collision avoidance in multi-robot navigation problem \cite{reif1999social, balch2000social, gayle2009multi}, these approaches are simple to implement but difficult to deal with local minima.

In general, most of methods simply treats the other robots which could make decision independently to avoid collision as dynamic obstacles so that the reciprocity between robots is overlooked.
these approaches could predict the collision regions for robots and select the velocity which could avoid reaching the union of these collision regions for each robot in real time, however, 
To summarize, few works choose polytopic robots as the research target, and the reliable real-time collision avoidance in navigation of distributed multi polytopic robots system is still a challenging problem.
